# Supplementary material for: Learning from Humans for Proactive Assistance in Human-Robot Collaborative Transport
Source: arXiv:2609.25351 source file (2026-09-21)
Supplement: Supplementary file 1 [file 08-appendix.tex]

\section{Appendix}

\subsection{Implementation Details}

All training and evaluation was performed on a system with an Intel i7-13700 CPU and an Nvidia GeForce RTX 4090 GPU.

We downsampled object poses from motion capture to 20 Hz based on empirical results to supply commands at a high enough control rate while smoothing noise in the derived object twists.

We run the low-level controller at \qty{500}{\hertz} to match the native control rate of the UR10e.
The low-level controller has a profiled median runtime of \qty{0.3}{\milli\second}, leaving computational headroom relative to the \qty{2}{\milli\second} control period.


\begin{table}
    \centering
    \caption{Learned model parameters at deployment.}
    \begin{tabular}{ll}
        \toprule
        Parameter & Value \\
        \midrule
        \hist & 60 (\qty{3}{\second}) \\
        \pred & 20 (\qty{1}{\second}) \\
        \refPathLen     & 12 (\qty{1.2}{\m}) \\
        Encoding dim & 256 \\
        Attention heads & 8 \\
        Feedforward dim & 512 \\
        Encoding layers & 4 \\
        Epochs & 50 \\
        Dropout & 0.1 \\
        Learning rate & 1e-3 \\
        Loss Function & SmoothL1 \\
        Optimizer & AdamW \\
        LR Scheduler & cosine \\
        LR Warmup Epochs & 5 \\
        \bottomrule
    \end{tabular}
\end{table}
